# Supplementary material for: ChiseLLM: Unleashing the Power of Reasoning LLMs for Chisel Agile Hardware Development
Source: arXiv:2504.19144 source file (2025-04-27)
Supplement: Supplementary file 1 [file appendix-experiment-setup.tex]

\section{Experiment Setup}
\label{sec:appendix-experiment-setup}
