# Supplementary material for: ChiseLLM: Unleashing the Power of Reasoning LLMs for Chisel Agile Hardware Development
Source: arXiv:2504.19144 source file (2025-04-27)
Supplement: Supplementary file 2 [file appendix-impl-details.tex]

\section{Implementation Details}
\label{sec:appendix-impl-details}
