# Supplementary material for: ChiseLLM: Unleashing the Power of Reasoning LLMs for Chisel Agile Hardware Development
Source: arXiv:2504.19144 source file (2025-04-27)
Supplement: Supplementary file 3 [file appendix-training-config.tex]

\section{Training Configuration}
\label{sec:appendix-training-config}
